# Supplementary material for: Dynamical Masses and Mass-to-light Ratios of Resolved Massive Star Clusters. I. NGC 419 and NGC 1846
Source: arXiv:1909.02056 ancillary file (2019-09-04)
Supplement: Supplementary file 1 [file Tab4_Tab5_full.pdf]

**Table 4.** M2FS Sample of NGC 419

| ID          | $\alpha_{2000}$<br>(h:m:s) | $\delta_{2000}$<br>( $^{\circ}$ : $'$ : $''$ ) | $V$<br>(mag)       | $V - I$<br>(mag)  | $v_{\text{los}}$<br>( $\text{km s}^{-1}$ ) | $P_{M_i}$ | Sel. <sup>a</sup> |
|-------------|----------------------------|------------------------------------------------|--------------------|-------------------|--------------------------------------------|-----------|-------------------|
| N419-1-b001 | 01:08:44.19                | -73:00:40.0                                    | $16.887 \pm 0.047$ | $1.497 \pm 0.055$ | $188.41 \pm 0.20$                          | 0.00      | M                 |
| N419-1-b002 | 01:08:46.07                | -72:56:35.2                                    | $17.942 \pm 0.030$ | $1.024 \pm 0.056$ | $192.79 \pm 0.42$                          | 0.00      | M                 |
| N419-1-b003 | 01:08:45.46                | -72:55:15.4                                    | $17.982 \pm 0.030$ | $1.138 \pm 0.043$ | $153.30 \pm 0.39$                          | 0.00      | M                 |
| N419-1-b004 | 01:08:43.26                | -72:53:32.0                                    | $18.014 \pm 0.008$ | $0.855 \pm 0.010$ | $193.60 \pm 0.61$                          | 0.06      | H                 |
| N419-1-b005 | 01:08:42.25                | -72:53:12.3                                    | $18.769 \pm 0.010$ | $1.019 \pm 0.013$ | $144.09 \pm 1.05$                          | 0.00      | H                 |
| N419-1-b006 | 01:08:36.93                | -72:53:08.6                                    | $18.072 \pm 0.007$ | $1.153 \pm 0.009$ | $188.79 \pm 0.36$                          | 0.95      | H                 |
| N419-1-b007 | 01:08:45.63                | -72:53:00.6                                    | $16.447 \pm 0.005$ | $1.721 \pm 0.005$ | $188.41 \pm 0.19$                          | 0.89      | H                 |
| N419-1-b008 | 01:08:42.71                | -72:52:36.2                                    | $18.742 \pm 0.012$ | $1.156 \pm 0.014$ | $163.46 \pm 0.75$                          | 0.00      | H                 |
| N419-1-b009 | 01:08:46.44                | -72:59:58.8                                    | $18.888 \pm 0.090$ | $0.809 \pm 0.139$ | $147.99 \pm 2.12$                          | 0.00      | M                 |
| N419-1-b010 | 01:08:53.00                | -72:59:08.5                                    | $18.126 \pm 0.074$ | $1.334 \pm 0.113$ | $191.09 \pm 0.88$                          | 0.00      | M                 |
| N419-1-b011 | 01:09:36.98                | -72:58:13.9                                    | $18.951 \pm 0.040$ | $0.873 \pm 0.058$ | $131.76 \pm 0.77$                          | 0.00      | M                 |
| N419-1-b012 | 01:09:10.13                | -72:57:30.3                                    | $16.764 \pm 0.108$ | $1.687 \pm 0.130$ | $171.52 \pm 0.27$                          | 0.00      | M                 |
| N419-1-b013 | 01:09:25.91                | -72:55:17.1                                    | $18.384 \pm 0.031$ | $1.030 \pm 0.054$ | $160.83 \pm 0.71$                          | 0.00      | M                 |
| N419-1-b015 | 01:08:52.25                | -72:53:57.3                                    | $18.896 \pm 0.088$ | $1.096 \pm 0.096$ | $134.17 \pm 0.93$                          | 0.00      | M                 |
| N419-1-b017 | 01:09:11.83                | -72:48:22.3                                    | $17.250 \pm 0.029$ | $1.316 \pm 0.039$ | $180.94 \pm 0.47$                          | 0.00      | M                 |
| N419-1-b018 | 01:09:03.45                | -72:50:13.0                                    | $18.416 \pm 0.119$ | $0.778 \pm 0.126$ | $204.86 \pm 1.45$                          | 0.00      | M                 |
| N419-1-b019 | 01:08:45.59                | -72:50:52.7                                    | $18.672 \pm 0.009$ | $1.140 \pm 0.011$ | $190.08 \pm 0.53$                          | 0.94      | H                 |
| N419-1-b020 | 01:08:40.43                | -72:51:00.7                                    | $17.596 \pm 0.007$ | $1.011 \pm 0.009$ | $187.88 \pm 0.33$                          | 0.70      | H                 |
| N419-1-b021 | 01:09:49.97                | -72:51:21.8                                    | $17.449 \pm 0.032$ | $1.404 \pm 0.043$ | $151.76 \pm 0.37$                          | 0.00      | M                 |
| N419-1-b022 | 01:08:42.54                | -72:51:27.5                                    | $18.392 \pm 0.009$ | $0.871 \pm 0.011$ | $146.39 \pm 0.58$                          | 0.00      | H                 |
| N419-1-b024 | 01:08:38.89                | -72:52:05.9                                    | $18.954 \pm 0.012$ | $1.048 \pm 0.014$ | $184.06 \pm 0.90$                          | 0.01      | H                 |
| N419-1-b025 | 01:08:33.04                | -72:50:58.4                                    | $17.834 \pm 0.009$ | $1.250 \pm 0.010$ | $190.24 \pm 0.30$                          | 0.93      | H                 |
| N419-1-b026 | 01:08:29.54                | -72:51:08.5                                    | $17.755 \pm 0.007$ | $0.905 \pm 0.009$ | $177.46 \pm 0.36$                          | 0.00      | H                 |
| N419-1-b027 | 01:08:33.47                | -72:51:17.0                                    | $18.714 \pm 0.009$ | $1.108 \pm 0.011$ | $112.31 \pm 0.63$                          | 0.00      | H                 |
| N419-1-b028 | 01:08:33.67                | -72:51:38.9                                    | $16.385 \pm 0.003$ | $1.766 \pm 0.004$ | $191.91 \pm 0.22$                          | 0.72      | H                 |
| N419-1-b029 | 01:08:38.81                | -72:51:45.7                                    | $16.818 \pm 0.004$ | $0.876 \pm 0.005$ | $146.89 \pm 0.27$                          | 0.00      | H                 |
| N419-1-b030 | 01:08:29.68                | -72:51:58.8                                    | $17.386 \pm 0.005$ | $1.340 \pm 0.006$ | $144.66 \pm 0.31$                          | 0.00      | H                 |
| N419-1-b031 | 01:08:35.45                | -72:52:05.2                                    | $18.612 \pm 0.008$ | $1.165 \pm 0.011$ | $132.97 \pm 0.63$                          | 0.00      | H                 |
| N419-1-b032 | 01:08:36.88                | -72:52:22.3                                    | $16.422 \pm 0.003$ | $1.680 \pm 0.004$ | $189.04 \pm 0.21$                          | 0.94      | H                 |
| N419-1-b033 | 01:08:28.67                | -72:59:24.5                                    | $18.561 \pm 0.036$ | $1.056 \pm 0.047$ | $172.83 \pm 0.56$                          | 0.00      | M                 |
| N419-1-b034 | 01:08:29.52                | -72:57:16.4                                    | $17.474 \pm 0.063$ | $1.323 \pm 0.115$ | $153.03 \pm 0.29$                          | 0.00      | M                 |
| N419-1-b035 | 01:08:27.14                | -72:54:05.2                                    | $17.010 \pm 0.005$ | $1.423 \pm 0.006$ | $188.55 \pm 0.22$                          | 0.99      | H                 |
| N419-1-b036 | 01:08:26.24                | -72:53:47.1                                    | $18.342 \pm 0.011$ | $1.124 \pm 0.015$ | $190.10 \pm 0.61$                          | 0.99      | H                 |
| N419-1-b037 | 01:08:30.79                | -72:53:30.9                                    | $17.477 \pm 0.005$ | $1.153 \pm 0.006$ | $188.48 \pm 0.29$                          | 0.98      | H                 |
| N419-1-b038 | 01:08:31.77                | -72:53:13.3                                    | $18.697 \pm 0.009$ | $0.946 \pm 0.012$ | $120.42 \pm 0.94$                          | 0.00      | H                 |
| N419-1-b039 | 01:08:28.43                | -72:53:12.6                                    | $18.621 \pm 0.009$ | $1.051 \pm 0.012$ | $187.58 \pm 0.79$                          | 0.99      | H                 |
| N419-1-b040 | 01:08:28.99                | -72:52:58.2                                    | $17.982 \pm 0.008$ | $1.163 \pm 0.009$ | $192.70 \pm 0.56$                          | 0.97      | H                 |
| N419-1-b041 | 01:08:33.26                | -73:00:25.3                                    | $17.997 \pm 0.106$ | $0.946 \pm 0.301$ | $189.95 \pm 0.46$                          | 0.00      | M                 |

*Table 4 continued*

Table 4 (continued)

| ID          | $\alpha_{2000}$<br>(h:m:s) | $\delta_{2000}$<br>( $^{\circ}$ : $'$ : $''$ ) | $V$<br>(mag)       | $V - I$<br>(mag)  | $v_{\text{los}}$<br>( $\text{km s}^{-1}$ ) | $P_{M_i}$ | Sel. <sup>a</sup> |
|-------------|----------------------------|------------------------------------------------|--------------------|-------------------|--------------------------------------------|-----------|-------------------|
| N419-1-b043 | 01:08:34.41                | -72:55:19.0                                    | 18.900 $\pm$ 0.042 | 1.034 $\pm$ 0.068 | 144.91 $\pm$ 1.60                          | 0.00      | M                 |
| N419-1-b046 | 01:08:34.51                | -72:52:59.8                                    | 15.918 $\pm$ 0.002 | 1.244 $\pm$ 0.003 | 182.92 $\pm$ 0.17                          | 0.00      | H                 |
| N419-1-b047 | 01:08:32.54                | -72:52:45.8                                    | 18.615 $\pm$ 0.010 | 1.082 $\pm$ 0.012 | 191.86 $\pm$ 0.70                          | 0.97      | H                 |
| N419-1-b048 | 01:08:36.71                | -72:52:40.4                                    | 18.329 $\pm$ 0.007 | 1.155 $\pm$ 0.009 | 171.83 $\pm$ 0.40                          | 0.00      | H                 |
| N419-1-b049 | 01:08:25.26                | -72:48:18.5                                    | 18.977 $\pm$ 0.044 | 0.885 $\pm$ 0.092 | 159.73 $\pm$ 1.57                          | 0.00      | M                 |
| N419-1-b050 | 01:08:22.58                | -72:51:11.8                                    | 18.949 $\pm$ 0.026 | 0.991 $\pm$ 0.032 | 139.76 $\pm$ 1.13                          | 0.00      | H                 |
| N419-1-b051 | 01:08:25.32                | -72:51:18.1                                    | 17.126 $\pm$ 0.007 | 1.438 $\pm$ 0.008 | 190.63 $\pm$ 0.35                          | 0.93      | H                 |
| N419-1-b052 | 01:08:22.12                | -72:51:37.8                                    | 17.296 $\pm$ 0.005 | 1.314 $\pm$ 0.006 | 197.80 $\pm$ 0.28                          | 0.00      | H                 |
| N419-1-b053 | 01:08:28.90                | -72:51:42.8                                    | 18.442 $\pm$ 0.012 | 0.855 $\pm$ 0.016 | 146.51 $\pm$ 1.03                          | 0.00      | H                 |
| N419-1-b055 | 01:08:24.75                | -72:52:25.3                                    | 17.717 $\pm$ 0.008 | 1.107 $\pm$ 0.010 | 192.58 $\pm$ 0.45                          | 0.98      | H                 |
| N419-1-b057 | 01:08:16.73                | -72:51:29.0                                    | 17.752 $\pm$ 0.008 | 1.364 $\pm$ 0.009 | 139.19 $\pm$ 0.33                          | 0.00      | H                 |
| N419-1-b058 | 01:08:17.65                | -72:51:52.8                                    | 16.563 $\pm$ 0.003 | 1.566 $\pm$ 0.004 | 188.98 $\pm$ 0.20                          | 0.99      | H                 |
| N419-1-b059 | 01:08:21.63                | -72:52:00.7                                    | 18.862 $\pm$ 0.010 | 0.958 $\pm$ 0.013 | 190.29 $\pm$ 1.00                          | 0.99      | H                 |
| N419-1-b061 | 01:08:20.37                | -72:52:22.1                                    | 16.785 $\pm$ 0.004 | 1.496 $\pm$ 0.004 | 188.40 $\pm$ 0.25                          | 1.00      | H                 |
| N419-1-b063 | 01:08:13.56                | -72:52:40.1                                    | 18.429 $\pm$ 0.008 | 1.051 $\pm$ 0.010 | 190.22 $\pm$ 1.38                          | 1.00      | H                 |
| N419-1-b064 | 01:08:17.60                | -72:52:48.4                                    | 18.092 $\pm$ 0.008 | 1.183 $\pm$ 0.009 | 189.78 $\pm$ 2.07                          | 1.00      | H                 |
| N419-1-b065 | 01:08:13.57                | -72:54:31.7                                    | 18.633 $\pm$ 0.010 | 1.140 $\pm$ 0.013 | 175.23 $\pm$ 0.69                          | 0.00      | H                 |
| N419-1-b066 | 01:08:10.42                | -72:54:16.5                                    | 18.245 $\pm$ 0.009 | 1.176 $\pm$ 0.011 | 142.15 $\pm$ 0.57                          | 0.00      | H                 |
| N419-1-b067 | 01:08:17.34                | -72:54:12.7                                    | 17.027 $\pm$ 0.008 | 1.445 $\pm$ 0.011 | 190.42 $\pm$ 0.35                          | 0.99      | H                 |
| N419-1-b069 | 01:08:14.49                | -72:53:31.4                                    | 17.865 $\pm$ 0.006 | 1.163 $\pm$ 0.008 | 187.93 $\pm$ 0.63                          | 1.00      | H                 |
| N419-1-b070 | 01:08:10.48                | -72:53:27.3                                    | 19.161 $\pm$ 0.010 | 0.916 $\pm$ 0.014 | 185.28 $\pm$ 1.45                          | 1.00      | H                 |
| N419-1-b071 | 01:08:14.04                | -72:53:16.4                                    | 16.573 $\pm$ 0.003 | 1.564 $\pm$ 0.004 | 187.81 $\pm$ 0.37                          | 1.00      | H                 |
| N419-1-b074 | 01:08:25.83                | -72:54:19.8                                    | 18.574 $\pm$ 0.013 | 1.063 $\pm$ 0.017 | 189.96 $\pm$ 0.68                          | 0.96      | H                 |
| N419-1-b075 | 01:08:21.22                | -72:54:03.6                                    | 17.017 $\pm$ 0.004 | 1.573 $\pm$ 0.005 | 161.88 $\pm$ 0.30                          | 0.00      | H                 |
| N419-1-b077 | 01:08:22.33                | -72:53:40.0                                    | 19.442 $\pm$ 0.015 | 0.903 $\pm$ 0.019 | 186.61 $\pm$ 1.99                          | 1.00      | H                 |
| N419-1-b078 | 01:08:24.57                | -72:53:28.2                                    | 17.418 $\pm$ 0.005 | 1.245 $\pm$ 0.006 | 189.61 $\pm$ 0.34                          | 1.00      | H                 |
| N419-1-b079 | 01:08:18.45                | -72:53:15.9                                    | 16.921 $\pm$ 0.004 | 1.387 $\pm$ 0.005 | 188.15 $\pm$ 0.51                          | 1.00      | H                 |
| N419-1-b080 | 01:08:19.35                | -72:53:00.9                                    | 16.422 $\pm$ 0.003 | 1.682 $\pm$ 0.004 | 189.50 $\pm$ 0.62                          | 1.00      | H                 |
| N419-1-b081 | 01:08:10.72                | -72:49:08.4                                    | 16.956 $\pm$ 0.033 | 1.321 $\pm$ 0.276 | 123.35 $\pm$ 0.36                          | 0.00      | M                 |
| N419-1-b082 | 01:08:13.42                | -72:51:11.0                                    | 18.842 $\pm$ 0.011 | 1.071 $\pm$ 0.014 | 189.78 $\pm$ 0.93                          | 0.94      | H                 |
| N419-1-b083 | 01:08:10.12                | -72:51:21.7                                    | 18.596 $\pm$ 0.009 | 1.093 $\pm$ 0.012 | 117.91 $\pm$ 0.85                          | 0.00      | H                 |
| N419-1-b084 | 01:08:12.53                | -72:51:30.2                                    | 17.660 $\pm$ 0.006 | 1.187 $\pm$ 0.007 | 191.81 $\pm$ 0.29                          | 0.80      | H                 |
| N419-1-b086 | 01:08:12.85                | -72:52:25.0                                    | 18.587 $\pm$ 0.009 | 0.880 $\pm$ 0.012 | 146.58 $\pm$ 1.76                          | 0.00      | H                 |
| N419-1-b087 | 01:08:09.31                | -72:52:37.5                                    | 16.944 $\pm$ 0.005 | 1.323 $\pm$ 0.006 | 192.62 $\pm$ 0.34                          | 0.98      | H                 |
| N419-1-b088 | 01:08:09.87                | -72:52:54.5                                    | 16.992 $\pm$ 0.005 | 1.413 $\pm$ 0.006 | 188.23 $\pm$ 0.32                          | 1.00      | H                 |
| N419-1-b089 | 01:08:06.74                | -72:51:17.8                                    | 18.399 $\pm$ 0.011 | 1.073 $\pm$ 0.014 | 189.03 $\pm$ 0.50                          | 0.94      | H                 |
| N419-1-b091 | 01:08:05.25                | -72:51:52.7                                    | 18.349 $\pm$ 0.007 | 1.069 $\pm$ 0.009 | 168.13 $\pm$ 0.78                          | 0.00      | H                 |
| N419-1-b092 | 01:08:08.77                | -72:51:55.3                                    | 19.021 $\pm$ 0.012 | 0.840 $\pm$ 0.016 | 184.36 $\pm$ 2.47                          | 0.87      | H                 |
| N419-1-b093 | 01:08:04.31                | -72:52:09.6                                    | 17.011 $\pm$ 0.005 | 1.323 $\pm$ 0.006 | 187.75 $\pm$ 0.24                          | 0.97      | H                 |
| N419-1-b094 | 01:08:05.31                | -72:52:30.0                                    | 16.772 $\pm$ 0.004 | 0.914 $\pm$ 0.005 | 157.41 $\pm$ 0.29                          | 0.00      | H                 |

Table 4 continued

Table 4 (continued)

| ID          | $\alpha_{2000}$<br>(h:m:s) | $\delta_{2000}$<br>( $^{\circ}$ : $'$ : $''$ ) | $V$<br>(mag)       | $V - I$<br>(mag)  | $v_{\text{los}}$<br>( $\text{km s}^{-1}$ ) | $P_{M_i}$ | Sel. <sup>a</sup> |
|-------------|----------------------------|------------------------------------------------|--------------------|-------------------|--------------------------------------------|-----------|-------------------|
| N419-1-b095 | 01:08:06.26                | -72:52:55.3                                    | $19.328 \pm 0.015$ | $0.901 \pm 0.019$ | $172.96 \pm 2.16$                          | 0.00      | H                 |
| N419-1-b096 | 01:08:07.57                | -72:53:10.7                                    | $17.097 \pm 0.006$ | $1.412 \pm 0.007$ | $188.48 \pm 0.24$                          | 0.99      | H                 |
| N419-1-b097 | 01:07:34.42                | -72:57:42.7                                    | $17.215 \pm 0.030$ | $0.956 \pm 0.055$ | $159.54 \pm 0.32$                          | 0.00      | M                 |
| N419-1-b098 | 01:07:33.01                | -72:57:06.7                                    | $16.802 \pm 0.050$ | $1.732 \pm 0.060$ | $175.10 \pm 0.27$                          | 0.00      | M                 |
| N419-1-b099 | 01:07:32.16                | -72:56:45.0                                    | $16.907 \pm 0.037$ | $1.542 \pm 0.129$ | $168.45 \pm 0.24$                          | 0.00      | M                 |
| N419-1-b100 | 01:07:46.32                | -72:56:03.5                                    | $17.036 \pm 0.033$ | $1.016 \pm 0.102$ | $191.41 \pm 0.25$                          | 0.00      | M                 |
| N419-1-b101 | 01:07:24.42                | -72:55:21.7                                    | $18.252 \pm 0.108$ | $1.212 \pm 0.122$ | $161.95 \pm 0.54$                          | 0.00      | M                 |
| N419-1-b102 | 01:06:54.30                | -72:55:17.1                                    | $17.468 \pm 0.029$ | $1.286 \pm 0.040$ | $146.65 \pm 0.37$                          | 0.00      | M                 |
| N419-1-b103 | 01:06:38.13                | -72:55:16.4                                    | $17.603 \pm 0.036$ | $1.365 \pm 0.271$ | $190.53 \pm 0.38$                          | 0.00      | M                 |
| N419-1-b104 | 01:07:31.81                | -72:54:00.3                                    | $17.507 \pm 0.187$ | $0.884 \pm 0.236$ | $151.85 \pm 0.37$                          | 0.00      | M                 |
| N419-1-b105 | 01:08:03.10                | -73:00:02.7                                    | $17.691 \pm 0.030$ | $1.408 \pm 0.077$ | $148.05 \pm 0.42$                          | 0.00      | M                 |
| N419-1-b106 | 01:07:51.35                | -72:58:01.4                                    | $18.800 \pm 0.102$ | $0.896 \pm 0.111$ | $182.85 \pm 1.67$                          | 0.00      | M                 |
| N419-1-b107 | 01:08:07.38                | -72:54:09.8                                    | $18.579 \pm 0.011$ | $1.129 \pm 0.013$ | $158.16 \pm 0.67$                          | 0.00      | H                 |
| N419-1-b109 | 01:08:06.35                | -72:53:32.4                                    | $16.666 \pm 0.004$ | $1.495 \pm 0.004$ | $190.11 \pm 0.24$                          | 0.99      | H                 |
| N419-1-b110 | 01:08:02.42                | -72:53:27.6                                    | $18.188 \pm 0.010$ | $1.140 \pm 0.013$ | $188.10 \pm 0.51$                          | 0.98      | H                 |
| N419-1-b111 | 01:08:04.02                | -72:53:10.5                                    | $17.301 \pm 0.007$ | $1.359 \pm 0.008$ | $190.28 \pm 0.34$                          | 0.99      | H                 |
| N419-1-b112 | 01:08:02.60                | -72:52:56.9                                    | $18.781 \pm 0.010$ | $1.011 \pm 0.013$ | $189.47 \pm 0.92$                          | 0.99      | H                 |
| N419-1-b114 | 01:07:51.42                | -72:50:55.6                                    | $16.972 \pm 0.029$ | $1.503 \pm 0.151$ | $161.58 \pm 0.25$                          | 0.00      | M                 |
| N419-1-b115 | 01:08:01.76                | -72:51:30.5                                    | $18.893 \pm 0.015$ | $0.797 \pm 0.018$ | $172.99 \pm 1.39$                          | 0.00      | H                 |
| N419-1-b117 | 01:07:29.46                | -72:52:04.5                                    | $18.969 \pm 0.036$ | $0.839 \pm 0.073$ | $131.08 \pm 1.48$                          | 0.00      | M                 |
| N419-1-b118 | 01:08:03.20                | -72:52:40.0                                    | $17.869 \pm 0.007$ | $1.142 \pm 0.009$ | $191.56 \pm 0.39$                          | 0.98      | H                 |
| N419-1-b119 | 01:07:53.96                | -72:54:06.2                                    | $18.464 \pm 0.031$ | $1.001 \pm 0.051$ | $159.17 \pm 0.50$                          | 0.00      | M                 |
| N419-1-b120 | 01:07:59.08                | -72:54:49.3                                    | $17.269 \pm 0.040$ | $1.394 \pm 0.056$ | $136.46 \pm 0.21$                          | 0.00      | M                 |
| N419-1-b121 | 01:07:30.01                | -72:49:42.7                                    | $17.971 \pm 0.031$ | $1.029 \pm 0.042$ | $142.66 \pm 0.65$                          | 0.00      | M                 |
| N419-1-b123 | 01:07:10.06                | -72:50:32.3                                    | $18.746 \pm 0.055$ | $0.889 \pm 0.091$ | $191.94 \pm 1.46$                          | 0.00      | M                 |
| N419-1-b124 | 01:07:22.03                | -72:50:49.3                                    | $18.413 \pm 0.036$ | $1.115 \pm 0.047$ | $166.43 \pm 0.60$                          | 0.00      | M                 |
| N419-1-b126 | 01:06:48.72                | -72:53:33.3                                    | $16.916 \pm 0.028$ | $1.015 \pm 0.040$ | $149.91 \pm 0.29$                          | 0.00      | M                 |
| N419-1-b127 | 01:06:36.00                | -72:54:14.6                                    | $17.088 \pm 0.032$ | $1.284 \pm 0.049$ | $141.47 \pm 1.12$                          | 0.00      | M                 |
| N419-1-b128 | 01:06:59.45                | -72:54:39.6                                    | $16.997 \pm 0.030$ | $1.372 \pm 0.064$ | $142.84 \pm 0.28$                          | 0.00      | M                 |
| N419-1-r049 | 01:08:14.47                | -72:53:56.6                                    | $16.214 \pm 0.004$ | $1.934 \pm 0.004$ | $186.85 \pm 0.36$                          | 0.97      | H                 |
| N419-1-r079 | 01:08:20.73                | -72:52:47.2                                    | $16.342 \pm 0.003$ | $1.762 \pm 0.004$ | $193.99 \pm 0.29$                          | 1.00      | H                 |
| N419-1-r099 | 01:08:26.87                | -72:52:46.3                                    | $16.523 \pm 0.004$ | $1.661 \pm 0.004$ | $191.02 \pm 0.24$                          | 0.99      | H                 |
| N419-1-r127 | 01:08:23.70                | -72:53:09.1                                    | $16.312 \pm 0.003$ | $1.741 \pm 0.004$ | $187.89 \pm 0.40$                          | 1.00      | H                 |

<sup>a</sup>Photometric source that the target were selected from: H stands for *HST* and M stands for MCPS.

**Table 5.** Combined Sample of NGC 1846

| ID           | $\alpha_{2000}$<br>(h:m:s) | $\delta_{2000}$<br>(°:':") | $V$<br>(mag)   | $V - I$<br>(mag) | $v_{\text{los}}$<br>(km s <sup>-1</sup> ) | $P_{M_i}$ | Sel. <sup>a</sup> | Spec. <sup>b</sup> |
|--------------|----------------------------|----------------------------|----------------|------------------|-------------------------------------------|-----------|-------------------|--------------------|
| N1846-1-b001 | 05:07:51.21                | -67:33:03.8                | 17.251 ± 0.307 | 1.396 ± 0.310    | 287.97 ± 0.19                             | 0.00      | M                 | M2FS               |
| N1846-1-b002 | 05:07:57.56                | -67:32:58.0                | 17.314 ± 0.049 | 1.266 ± 0.069    | 264.51 ± 0.19                             | 0.00      | M                 | M2FS               |
| N1846-1-b003 | 05:07:49.91                | -67:32:21.2                | 17.559 ± 0.041 | 1.255 ± 0.058    | 246.95 ± 0.18                             | 0.00      | M                 | M2FS               |
| N1846-1-b005 | 05:07:54.32                | -67:30:17.6                | 17.715 ± 0.030 | 1.192 ± 0.050    | 221.35 ± 0.23                             | 0.00      | M                 | M2FS               |
| N1846-1-b006 | 05:07:47.87                | -67:29:52.6                | 17.329 ± 0.028 | 1.345 ± 0.049    | 271.34 ± 0.19                             | 0.00      | M                 | M2FS               |
| N1846-1-b007 | 05:07:56.92                | -67:29:28.9                | 17.387 ± 0.146 | 1.256 ± 0.151    | 286.79 ± 0.20                             | 0.00      | M                 | M2FS               |
| N1846-1-b009 | 05:08:21.28                | -67:31:11.1                | 17.125 ± 0.026 | 1.301 ± 0.049    | 287.38 ± 0.17                             | 0.00      | M                 | M2FS               |
| N1846-1-b010 | 05:08:29.24                | -67:31:03.5                | 17.475 ± 0.050 | 1.278 ± 0.071    | 231.89 ± 0.18                             | 0.00      | M                 | M2FS               |
| N1846-1-b011 | 05:08:24.35                | -67:30:58.2                | 17.212 ± 0.054 | 1.304 ± 0.067    | 275.75 ± 0.18                             | 0.00      | M                 | M2FS               |
| N1846-1-b012 | 05:08:30.22                | -67:30:34.4                | 17.595 ± 0.060 | 1.194 ± 0.076    | 274.73 ± 0.19                             | 0.00      | M                 | M2FS               |
| N1846-1-b013 | 05:08:10.21                | -67:29:55.3                | 17.508 ± 0.038 | 1.348 ± 0.055    | 216.72 ± 0.20                             | 0.00      | M                 | M2FS               |
| N1846-1-b015 | 05:08:34.55                | -67:29:23.9                | 17.601 ± 0.031 | 1.284 ± 0.051    | 271.05 ± 0.20                             | 0.00      | M                 | M2FS               |
| N1846-1-b016 | 05:08:44.83                | -67:29:05.7                | 17.668 ± 0.043 | 1.178 ± 0.069    | 273.20 ± 0.21                             | 0.00      | M                 | M2FS               |
| N1846-1-b017 | 05:08:18.68                | -67:24:42.1                | 17.657 ± 0.031 | 1.293 ± 0.051    | 272.52 ± 0.24                             | 0.00      | M                 | M2FS               |
| N1846-1-b019 | 05:08:39.28                | -67:25:53.4                | 17.271 ± 0.023 | 1.354 ± 0.046    | 318.50 ± 0.14                             | 0.00      | M                 | M2FS               |
| N1846-1-b020 | 05:08:16.63                | -67:27:13.4                | 17.627 ± 0.039 | 1.228 ± 0.078    | 274.40 ± 0.15                             | 0.00      | M                 | M2FS               |
| N1846-1-b021 | 05:08:41.57                | -67:27:26.0                | 17.651 ± 0.053 | 1.184 ± 0.071    | 308.68 ± 0.30                             | 0.00      | M                 | M2FS               |
| N1846-1-b022 | 05:08:39.60                | -67:27:39.3                | 17.530 ± 0.031 | 1.297 ± 0.054    | 276.49 ± 0.19                             | 0.00      | M                 | M2FS               |
| N1846-1-b023 | 05:08:17.46                | -67:27:44.8                | 17.106 ± 0.027 | 1.295 ± 0.048    | 277.78 ± 0.15                             | 0.00      | M                 | M2FS               |
| N1846-1-b025 | 05:08:08.02                | -67:22:52.5                | 17.726 ± 0.242 | 1.295 ± 0.246    | 228.47 ± 0.21                             | 0.00      | M                 | M2FS               |
| N1846-1-b027 | 05:08:10.54                | -67:24:20.9                | 17.619 ± 0.031 | 1.180 ± 0.051    | 249.71 ± 0.20                             | 0.00      | M                 | M2FS               |
| N1846-1-b030 | 05:07:50.87                | -67:26:13.7                | 17.515 ± 0.031 | 1.283 ± 0.051    | 268.99 ± 0.19                             | 0.00      | M                 | M2FS               |
| N1846-1-b031 | 05:08:08.63                | -67:26:24.4                | 17.135 ± 0.031 | 1.323 ± 0.051    | 281.85 ± 0.14                             | 0.00      | M                 | M2FS               |
| N1846-1-b032 | 05:08:06.22                | -67:27:24.2                | 17.569 ± 0.035 | 1.327 ± 0.055    | 256.58 ± 0.19                             | 0.00      | M                 | M2FS               |
| N1846-1-b033 | 05:07:36.65                | -67:30:16.5                | 18.191 ± 0.008 | 1.141 ± 0.012    | 284.64 ± 0.32                             | 0.00      | H                 | M2FS               |
| N1846-1-b034 | 05:07:39.86                | -67:29:04.6                | 17.828 ± 0.031 | 1.140 ± 0.074    | 239.85 ± 0.27                             | 0.96      | M                 | M2FS               |
| N1846-1-b035 | 05:07:40.01                | -67:28:31.2                | 17.944 ± 0.006 | 1.164 ± 0.010    | 237.57 ± 0.23                             | 0.99      | H                 | M2FS               |
| N1846-1-b036 | 05:07:38.41                | -67:28:11.9                | 17.097 ± 0.004 | 1.431 ± 0.006    | 237.02 ± 0.18                             | 1.00      | H                 | COMB               |
| N1846-1-b037 | 05:07:36.12                | -67:28:07.8                | 17.872 ± 0.006 | 1.223 ± 0.009    | 238.59 ± 0.21                             | 1.00      | H                 | M2FS               |
| N1846-1-b038 | 05:07:38.15                | -67:27:58.7                | 17.345 ± 0.005 | 1.346 ± 0.007    | 237.39 ± 0.22                             | 1.00      | H                 | M2FS               |
| N1846-1-b039 | 05:07:39.58                | -67:27:38.2                | 17.223 ± 0.006 | 1.368 ± 0.008    | 238.69 ± 0.21                             | 1.00      | H                 | M2FS               |
| N1846-1-b043 | 05:07:42.35                | -67:28:46.1                | 18.248 ± 0.008 | 1.069 ± 0.015    | 245.91 ± 0.54                             | 0.00      | H                 | M2FS               |
| N1846-1-b044 | 05:07:45.51                | -67:28:34.2                | 18.077 ± 0.008 | 1.130 ± 0.012    | 264.15 ± 0.23                             | 0.00      | H                 | M2FS               |
| N1846-1-b045 | 05:07:47.37                | -67:28:19.8                | 17.580 ± 0.007 | 1.191 ± 0.011    | 236.37 ± 0.29                             | 0.61      | H                 | M2FS               |
| N1846-1-b046 | 05:07:44.74                | -67:28:18.5                | 17.078 ± 0.005 | 1.378 ± 0.007    | 237.50 ± 0.17                             | 0.99      | H                 | M2FS               |
| N1846-1-b047 | 05:07:43.71                | -67:27:58.4                | 18.138 ± 0.008 | 1.119 ± 0.012    | 238.06 ± 0.29                             | 1.00      | H                 | M2FS               |
| N1846-1-b048 | 05:07:41.77                | -67:27:51.3                | 18.301 ± 0.008 | 1.119 ± 0.012    | 240.36 ± 0.32                             | 1.00      | H                 | M2FS               |
| N1846-1-b049 | 05:07:42.99                | -67:21:35.8                | 17.481 ± 0.031 | 1.321 ± 0.040    | 271.34 ± 0.25                             | 0.00      | M                 | M2FS               |
| N1846-1-b050 | 05:07:45.88                | -67:23:42.5                | 17.471 ± 0.034 | 1.260 ± 0.110    | 282.03 ± 0.21                             | 0.00      | M                 | M2FS               |

*Table 5 continued*

Table 5 (continued)

| ID           | $\alpha_{2000}$<br>(h:m:s) | $\delta_{2000}$<br>(°:':") | $V$<br>(mag)   | $V - I$<br>(mag) | $v_{\text{los}}$<br>(km s <sup>-1</sup> ) | $P_{M_i}$ | Sel. <sup>a</sup> | Spec. <sup>b</sup> |
|--------------|----------------------------|----------------------------|----------------|------------------|-------------------------------------------|-----------|-------------------|--------------------|
| N1846-1-b052 | 05:07:47.67                | -67:26:05.6                | 17.546 ± 0.033 | 1.317 ± 0.053    | 236.68 ± 0.21                             | 0.27      | M                 | M2FS               |
| N1846-1-b053 | 05:07:41.62                | -67:26:27.4                | 18.302 ± 0.050 | 1.107 ± 0.068    | 280.18 ± 0.31                             | 0.00      | M                 | M2FS               |
| N1846-1-b054 | 05:07:37.75                | -67:26:51.9                | 17.956 ± 0.006 | 1.135 ± 0.012    | 237.89 ± 0.27                             | 1.00      | H                 | M2FS               |
| N1846-1-b055 | 05:07:39.46                | -67:26:59.9                | 18.292 ± 0.006 | 1.086 ± 0.011    | 238.90 ± 0.28                             | 1.00      | H                 | M2FS               |
| N1846-1-b056 | 05:07:40.73                | -67:27:22.2                | 17.760 ± 0.005 | 1.148 ± 0.009    | 239.49 ± 0.22                             | 1.00      | H                 | M2FS               |
| N1846-1-b057 | 05:07:33.97                | -67:22:12.1                | 17.608 ± 0.043 | 1.266 ± 0.050    | 240.19 ± 0.25                             | 0.00      | M                 | M2FS               |
| N1846-1-b058 | 05:07:32.31                | -67:26:35.3                | 17.770 ± 0.007 | 1.182 ± 0.010    | 239.90 ± 0.22                             | 1.00      | H                 | M2FS               |
| N1846-1-b059 | 05:07:32.45                | -67:26:49.6                | 17.398 ± 0.008 | 1.252 ± 0.010    | 240.29 ± 0.26                             | 1.00      | H                 | M2FS               |
| N1846-1-b061 | 05:07:34.81                | -67:26:53.6                | 17.504 ± 0.010 | 1.249 ± 0.012    | 241.38 ± 0.21                             | 1.00      | H                 | M2FS               |
| N1846-1-b062 | 05:07:34.27                | -67:27:13.7                | 17.541 ± 0.005 | 1.305 ± 0.008    | 243.18 ± 0.23                             | 0.99      | H                 | M2FS               |
| N1846-1-b063 | 05:07:36.86                | -67:27:19.2                | 18.201 ± 0.006 | 1.127 ± 0.011    | 242.08 ± 0.24                             | 1.00      | H                 | M2FS               |
| N1846-1-b064 | 05:07:34.23                | -67:27:27.0                | 17.624 ± 0.007 | 1.197 ± 0.009    | 239.50 ± 0.31                             | 1.00      | H                 | M2FS               |
| N1846-1-b065 | 05:07:22.62                | -67:33:31.4                | 17.170 ± 0.048 | 1.340 ± 0.070    | 314.15 ± 0.19                             | 0.00      | M                 | M2FS               |
| N1846-1-b066 | 05:07:28.51                | -67:32:40.7                | 17.527 ± 0.031 | 1.225 ± 0.061    | 268.08 ± 0.29                             | 0.00      | M                 | M2FS               |
| N1846-1-b067 | 05:07:29.05                | -67:31:58.0                | 17.503 ± 0.033 | 1.354 ± 0.053    | 290.41 ± 0.85                             | 0.00      | M                 | M2FS               |
| N1846-1-b068 | 05:07:30.38                | -67:29:36.0                | 17.617 ± 0.006 | 1.237 ± 0.008    | 239.36 ± 0.16                             | 0.97      | H                 | COMB               |
| N1846-1-b069 | 05:07:27.44                | -67:29:27.9                | 17.881 ± 0.006 | 1.124 ± 0.010    | 238.88 ± 0.21                             | 0.97      | H                 | COMB               |
| N1846-1-b070 | 05:07:29.52                | -67:28:48.8                | 18.291 ± 0.008 | 1.158 ± 0.013    | 240.42 ± 0.32                             | 1.00      | H                 | M2FS               |
| N1846-1-b071 | 05:07:28.71                | -67:28:24.7                | 17.516 ± 0.007 | 1.199 ± 0.010    | 238.60 ± 0.19                             | 1.00      | H                 | COMB               |
| N1846-1-b072 | 05:07:26.13                | -67:28:08.3                | 17.878 ± 0.006 | 1.203 ± 0.009    | 240.45 ± 0.25                             | 1.00      | H                 | M2FS               |
| N1846-1-b073 | 05:07:32.70                | -67:30:37.3                | 18.404 ± 0.021 | 1.123 ± 0.025    | 272.60 ± 0.25                             | 0.00      | H                 | M2FS               |
| N1846-1-b074 | 05:07:32.36                | -67:29:22.1                | 18.387 ± 0.010 | 1.011 ± 0.016    | 286.00 ± 0.33                             | 0.00      | H                 | M2FS               |
| N1846-1-b075 | 05:07:31.11                | -67:29:06.2                | 18.162 ± 0.006 | 1.112 ± 0.011    | 237.78 ± 0.27                             | 0.92      | H                 | M2FS               |
| N1846-1-b076 | 05:07:34.98                | -67:28:54.9                | 17.514 ± 0.006 | 1.338 ± 0.009    | 281.13 ± 0.21                             | 0.00      | H                 | M2FS               |
| N1846-1-b077 | 05:07:34.52                | -67:28:24.5                | 17.849 ± 0.008 | 1.236 ± 0.011    | 239.55 ± 0.27                             | 1.00      | H                 | COMB               |
| N1846-1-b078 | 05:07:34.01                | -67:28:10.7                | 18.325 ± 0.006 | 1.051 ± 0.012    | 241.18 ± 0.36                             | 1.00      | H                 | M2FS               |
| N1846-1-b079 | 05:07:30.42                | -67:28:04.5                | 17.090 ± 0.005 | 1.367 ± 0.007    | 239.58 ± 0.17                             | 1.00      | H                 | COMB               |
| N1846-1-b080 | 05:07:34.59                | -67:27:55.7                | 17.289 ± 0.005 | 1.329 ± 0.007    | 259.98 ± 0.22                             | 0.00      | H                 | M2FS               |
| N1846-1-b081 | 05:07:27.72                | -67:20:59.1                | 17.354 ± 0.051 | 1.283 ± 0.058    | 272.38 ± 0.21                             | 0.00      | M                 | M2FS               |
| N1846-1-b082 | 05:07:29.23                | -67:25:09.4                | 17.542 ± 0.033 | 1.176 ± 0.055    | 273.57 ± 0.25                             | 0.00      | M                 | M2FS               |
| N1846-1-b083 | 05:07:29.61                | -67:26:27.7                | 17.914 ± 0.008 | 1.231 ± 0.011    | 242.93 ± 0.26                             | 0.33      | H                 | COMB               |
| N1846-1-b084 | 05:07:30.03                | -67:26:43.0                | 17.175 ± 0.005 | 1.341 ± 0.007    | 239.37 ± 0.18                             | 1.00      | H                 | COMB               |
| N1846-1-b085 | 05:07:29.78                | -67:26:57.3                | 18.303 ± 0.011 | 1.088 ± 0.015    | 238.90 ± 0.32                             | 1.00      | H                 | M2FS               |
| N1846-1-b087 | 05:07:32.10                | -67:27:20.1                | 17.303 ± 0.006 | 1.357 ± 0.008    | 239.89 ± 0.22                             | 1.00      | H                 | M2FS               |
| N1846-1-b088 | 05:07:27.74                | -67:27:30.5                | 17.389 ± 0.006 | 1.276 ± 0.008    | 238.90 ± 0.21                             | 1.00      | H                 | M2FS               |
| N1846-1-b089 | 05:07:27.31                | -67:23:08.7                | 17.222 ± 0.084 | 1.409 ± 0.142    | 209.72 ± 0.20                             | 0.00      | M                 | M2FS               |
| N1846-1-b090 | 05:07:23.74                | -67:26:32.8                | 17.862 ± 0.006 | 1.176 ± 0.010    | 271.38 ± 0.24                             | 0.00      | H                 | M2FS               |
| N1846-1-b092 | 05:07:23.62                | -67:26:50.9                | 17.337 ± 0.007 | 1.363 ± 0.009    | 263.45 ± 0.20                             | 0.00      | H                 | COMB               |
| N1846-1-b093 | 05:07:26.29                | -67:26:57.1                | 18.010 ± 0.006 | 1.167 ± 0.010    | 292.12 ± 0.26                             | 0.00      | H                 | COMB               |
| N1846-1-b094 | 05:07:21.17                | -67:27:01.6                | 17.157 ± 0.004 | 1.368 ± 0.006    | 249.96 ± 0.17                             | 0.00      | H                 | COMB               |

Table 5 continued

Table 5 (continued)

| ID           | $\alpha_{2000}$<br>(h:m:s) | $\delta_{2000}$<br>(°:′:″) | $V$<br>(mag)   | $V - I$<br>(mag) | $v_{\text{los}}$<br>(km s <sup>-1</sup> ) | $P_{M_i}$ | Sel. <sup>a</sup> | Spec. <sup>b</sup> |
|--------------|----------------------------|----------------------------|----------------|------------------|-------------------------------------------|-----------|-------------------|--------------------|
| N1846-1-b095 | 05:07:24.90                | -67:27:14.0                | 18.363 ± 0.008 | 1.023 ± 0.013    | 235.76 ± 0.29                             | 0.99      | H                 | M2FS               |
| N1846-1-b096 | 05:07:21.66                | -67:27:25.7                | 17.603 ± 0.005 | 1.270 ± 0.008    | 240.15 ± 0.21                             | 1.00      | H                 | COMB               |
| N1846-1-b097 | 05:06:41.49                | -67:30:29.3                | 17.523 ± 0.048 | 1.259 ± 0.069    | 264.60 ± 0.37                             | 0.00      | M                 | M2FS               |
| N1846-1-b098 | 05:07:04.08                | -67:30:27.1                | 17.316 ± 0.121 | 1.251 ± 0.127    | 315.36 ± 0.22                             | 0.00      | M                 | M2FS               |
| N1846-1-b099 | 05:06:26.99                | -67:29:46.2                | 17.652 ± 0.055 | 1.242 ± 0.071    | 250.96 ± 0.36                             | 0.00      | M                 | M2FS               |
| N1846-1-b100 | 05:07:06.54                | -67:29:29.4                | 17.172 ± 0.108 | 1.302 ± 0.116    | 316.04 ± 0.19                             | 0.00      | M                 | M2FS               |
| N1846-1-b101 | 05:07:14.70                | -67:29:16.2                | 17.535 ± 0.011 | 1.335 ± 0.013    | 280.36 ± 0.19                             | 0.00      | H                 | COMB               |
| N1846-1-b102 | 05:07:10.60                | -67:28:31.4                | 18.059 ± 0.008 | 1.166 ± 0.012    | 280.89 ± 0.25                             | 0.00      | H                 | COMB               |
| N1846-1-b103 | 05:07:12.27                | -67:28:03.4                | 18.374 ± 0.007 | 1.157 ± 0.011    | 277.60 ± 0.27                             | 0.00      | H                 | M2FS               |
| N1846-1-b104 | 05:07:14.42                | -67:27:48.4                | 18.118 ± 0.010 | 1.184 ± 0.013    | 290.83 ± 0.20                             | 0.00      | H                 | COMB               |
| N1846-1-b105 | 05:07:21.53                | -67:34:28.6                | 17.266 ± 0.036 | 1.396 ± 0.060    | 275.00 ± 0.27                             | 0.00      | M                 | M2FS               |
| N1846-1-b106 | 05:07:17.39                | -67:33:22.2                | 17.688 ± 0.037 | 1.215 ± 0.055    | 274.33 ± 0.24                             | 0.00      | M                 | M2FS               |
| N1846-1-b110 | 05:07:19.98                | -67:29:37.3                | 17.423 ± 0.004 | 1.340 ± 0.007    | 310.81 ± 0.15                             | 0.00      | H                 | COMB               |
| N1846-1-b111 | 05:07:22.21                | -67:28:01.1                | 18.459 ± 0.009 | 1.049 ± 0.015    | 240.13 ± 0.37                             | 1.00      | H                 | M2FS               |
| N1846-1-b112 | 05:07:21.79                | -67:27:48.3                | 17.254 ± 0.004 | 1.278 ± 0.006    | 240.07 ± 0.23                             | 1.00      | H                 | M2FS               |
| N1846-1-b114 | 05:07:14.72                | -67:22:39.4                | 17.653 ± 0.033 | 1.218 ± 0.054    | 288.47 ± 0.22                             | 0.00      | M                 | M2FS               |
| N1846-1-b118 | 05:07:20.90                | -67:25:42.3                | 17.657 ± 0.085 | 1.197 ± 0.095    | 239.63 ± 0.26                             | 0.96      | M                 | M2FS               |
| N1846-1-b119 | 05:07:19.94                | -67:26:33.8                | 17.607 ± 0.049 | 1.189 ± 0.075    | 234.77 ± 0.23                             | 0.00      | M                 | M2FS               |
| N1846-1-b120 | 05:07:17.91                | -67:27:12.2                | 17.388 ± 0.137 | 1.359 ± 0.143    | 239.45 ± 0.21                             | 0.96      | M                 | M2FS               |
| N1846-1-b121 | 05:06:59.17                | -67:23:06.7                | 17.024 ± 0.023 | 1.295 ± 0.080    | 251.92 ± 0.19                             | 0.00      | M                 | M2FS               |
| N1846-1-b122 | 05:06:32.56                | -67:24:21.3                | 17.646 ± 0.044 | 1.188 ± 0.063    | 245.75 ± 0.30                             | 0.00      | M                 | M2FS               |
| N1846-1-b123 | 05:06:58.93                | -67:24:28.2                | 17.437 ± 0.085 | 1.210 ± 0.105    | 250.13 ± 0.22                             | 0.00      | M                 | M2FS               |
| N1846-1-b126 | 05:06:31.87                | -67:26:14.9                | 17.533 ± 0.031 | 1.262 ± 0.052    | 214.26 ± 0.34                             | 0.00      | M                 | M2FS               |
| N1846-1-b127 | 05:06:48.68                | -67:27:11.0                | 17.611 ± 0.099 | 1.301 ± 0.109    | 250.71 ± 1.47                             | 0.00      | M                 | M2FS               |
| N1846-1-b128 | 05:06:39.18                | -67:27:36.1                | 17.460 ± 0.031 | 1.211 ± 0.053    | 289.27 ± 0.51                             | 0.00      | M                 | M2FS               |
| N1846-1-r049 | 05:07:32.21                | -67:27:51.6                | 17.154 ± 0.004 | 1.401 ± 0.006    | 241.93 ± 0.26                             | 1.00      | H                 | M2FS               |
| N1846-1-r079 | 05:07:30.12                | -67:27:27.7                | 17.115 ± 0.004 | 1.306 ± 0.006    | 238.29 ± 0.17                             | 1.00      | H                 | COMB               |
| N1846-1-r099 | 05:07:31.18                | -67:27:39.9                | 17.054 ± 0.004 | 1.422 ± 0.006    | 239.11 ± 0.19                             | 1.00      | H                 | M2FS               |
| N1846-1-r127 | 05:07:34.13                | -67:27:43.3                | 17.057 ± 0.004 | 1.336 ± 0.006    | 239.22 ± 0.20                             | 1.00      | H                 | M2FS               |
| ACS-001-R    | 05:07:36.84                | -67:27:45.9                | 16.56          | 1.70             | 236.11 ± 0.53                             | 1.00      | H                 | M13                |
| ACS-013-R    | 05:07:33.59                | -67:26:41.2                | 16.99          | 1.43             | 238.10 ± 0.46                             | 1.00      | H                 | M13                |
| ACS-019-R    | 05:07:14.49                | -67:28:16.4                | ...            | ...              | 278.73 ± 0.47                             | 0.00      | H                 | M13                |
| ACS-025-R    | 05:07:36.19                | -67:27:58.8                | 17.28          | 1.35             | 238.28 ± 0.49                             | 1.00      | H                 | M13                |
| ACS-030-R    | 05:07:39.01                | -67:28:23.2                | 17.43          | 1.31             | 240.65 ± 0.60                             | 1.00      | H                 | M13                |
| ACS-046-R    | 05:07:32.64                | -67:27:45.5                | 17.92          | 1.24             | 237.54 ± 0.62                             | 1.00      | H                 | M13                |
| ACS-051-R    | 05:07:36.60                | -67:27:33.5                | 17.96          | 1.25             | 235.60 ± 0.77                             | 1.00      | H                 | M13                |
| ACS-059-R    | 05:07:28.63                | -67:28:44.8                | 18.04          | 1.19             | 237.75 ± 0.77                             | 1.00      | H                 | M13                |
| ACS-066-R    | 05:07:49.57                | -67:29:01.4                | 18.18          | 1.18             | 239.43 ± 0.78                             | 0.96      | H                 | M13                |
| ACS-080-A    | 05:07:30.30                | -67:27:11.2                | 17.09          | 1.36             | 243.87 ± 0.47                             | 0.92      | H                 | M13                |
| ACS-090-A    | 05:07:30.17                | -67:27:46.1                | 17.53          | 1.24             | 238.02 ± 0.62                             | 1.00      | H                 | M13                |

Table 5 continued

Table 5 (continued)

| ID        | $\alpha_{2000}$<br>(h:m:s) | $\delta_{2000}$<br>(°:′:″) | $V$<br>(mag)   | $V - I$<br>(mag) | $v_{\text{los}}$<br>(km s <sup>-1</sup> ) | $P_{M_i}$ | Sel. <sup>a</sup> | Spec. <sup>b</sup> |
|-----------|----------------------------|----------------------------|----------------|------------------|-------------------------------------------|-----------|-------------------|--------------------|
| ACS-112-A | 05:07:43.29                | -67:26:49.9                | 18.02          | 1.12             | 239.80 ± 0.67                             | 0.96      | H                 | M13                |
| MCPS-007  | 05:05:34.36                | -67:26:34.2                | 16.810 ± 0.063 | 1.622 ± 0.079    | 253.77 ± 0.85                             | 0.00      | M                 | M13                |
| MCPS-010  | 05:05:40.15                | -67:24:55.8                | 16.820 ± 0.048 | 1.792 ± 0.063    | 265.39 ± 0.59                             | 0.00      | M                 | M13                |
| MCPS-016  | 05:05:48.25                | -67:26:42.0                | 16.622 ± 0.191 | 1.636 ± 0.195    | 277.40 ± 0.55                             | 0.00      | M                 | M13                |
| MCPS-017  | 05:05:48.26                | -67:34:31.0                | 16.868 ± 0.027 | 1.553 ± 0.047    | 305.87 ± 0.59                             | 0.00      | M                 | M13                |
| MCPS-018  | 05:05:49.11                | -67:24:18.3                | 16.586 ± 0.065 | 2.020 ± 0.076    | 271.71 ± 1.03                             | 0.00      | M                 | M13                |
| MCPS-021  | 05:05:55.85                | -67:36:24.1                | 17.015 ± 0.025 | 1.955 ± 0.052    | 258.14 ± 0.95                             | 0.00      | M                 | M13                |
| MCPS-022  | 05:05:56.49                | -67:34:03.0                | 16.537 ± 0.027 | 1.533 ± 0.047    | 279.70 ± 0.48                             | 0.00      | M                 | M13                |
| MCPS-023  | 05:05:56.77                | -67:31:03.9                | 16.619 ± 0.033 | 1.724 ± 0.053    | 250.79 ± 0.52                             | 0.00      | M                 | M13                |
| MCPS-026  | 05:06:01.14                | -67:25:34.9                | 16.452 ± 0.045 | 1.810 ± 0.060    | 298.23 ± 0.57                             | 0.00      | M                 | M13                |
| MCPS-027  | 05:06:03.18                | -67:28:46.3                | 16.855 ± 0.029 | 1.576 ± 0.049    | 279.19 ± 0.55                             | 0.00      | M                 | M13                |
| MCPS-029  | 05:06:04.64                | -67:34:09.3                | 16.687 ± 0.038 | 1.684 ± 0.064    | 234.91 ± 0.63                             | 0.00      | M                 | M13                |
| MCPS-031  | 05:06:06.29                | -67:33:19.8                | 16.406 ± 0.071 | 1.694 ± 0.087    | 285.55 ± 0.65                             | 0.00      | M                 | M13                |
| MCPS-033  | 05:06:07.79                | -67:30:26.5                | 16.857 ± 0.043 | 1.544 ± 0.059    | 270.06 ± 0.52                             | 0.00      | M                 | M13                |
| MCPS-035  | 05:06:12.98                | -67:28:56.5                | 16.732 ± 0.034 | 1.730 ± 0.055    | 259.76 ± 0.45                             | 0.00      | M                 | M13                |
| MCPS-038  | 05:06:16.30                | -67:30:11.6                | 16.652 ± 0.031 | 1.927 ± 0.049    | 235.10 ± 0.59                             | 0.00      | M                 | M13                |
| MCPS-040  | 05:06:17.30                | -67:31:45.0                | 16.762 ± 0.050 | 1.714 ± 0.066    | 278.87 ± 0.59                             | 0.00      | M                 | M13                |
| MCPS-042  | 05:06:21.14                | -67:19:38.1                | 16.737 ± 0.053 | 1.748 ± 0.058    | 298.96 ± 0.55                             | 0.00      | M                 | M13                |
| MCPS-043  | 05:06:22.02                | -67:28:51.5                | 16.834 ± 0.100 | 1.688 ± 0.107    | 264.66 ± 0.45                             | 0.00      | M                 | M13                |
| MCPS-044  | 05:06:26.23                | -67:21:24.0                | 16.601 ± 0.043 | 1.768 ± 0.051    | 278.44 ± 0.63                             | 0.00      | M                 | M13                |
| MCPS-045  | 05:06:26.70                | -67:29:36.1                | 16.463 ± 0.042 | 1.772 ± 0.057    | 311.54 ± 0.45                             | 0.00      | M                 | M13                |
| MCPS-047  | 05:06:29.38                | -67:32:50.0                | 16.731 ± 0.032 | 1.628 ± 0.050    | 257.38 ± 0.55                             | 0.00      | M                 | M13                |
| MCPS-048  | 05:06:29.78                | -67:23:06.5                | 16.635 ± 0.028 | 1.719 ± 0.050    | 273.60 ± 0.47                             | 0.00      | M                 | M13                |
| MCPS-049  | 05:06:30.15                | -67:29:54.4                | 16.547 ± 0.045 | 1.661 ± 0.065    | 252.78 ± 0.54                             | 0.00      | M                 | M13                |
| MCPS-050  | 05:06:32.18                | -67:21:02.1                | 16.887 ± 0.032 | 1.731 ± 0.051    | 261.66 ± 0.49                             | 0.00      | M                 | M13                |
| MCPS-051  | 05:06:34.01                | -67:37:13.8                | 16.689 ± 0.031 | 1.679 ± 0.051    | 279.60 ± 0.62                             | 0.00      | M                 | M13                |
| MCPS-052  | 05:06:34.74                | -67:21:09.6                | 16.317 ± 0.023 | 1.784 ± 0.033    | 235.45 ± 0.60                             | 0.00      | M                 | M13                |
| MCPS-058  | 05:06:40.72                | -67:37:16.7                | 15.643 ± 0.038 | 1.445 ± 0.055    | 298.75 ± 0.48                             | 0.00      | M                 | M13                |
| MCPS-059  | 05:06:40.76                | -67:16:24.3                | 17.147 ± 0.027 | 1.765 ± 0.036    | 324.81 ± 0.65                             | 0.00      | M                 | M13                |
| MCPS-060  | 05:06:42.46                | -67:32:28.6                | 16.804 ± 0.046 | 1.979 ± 0.060    | 248.33 ± 1.12                             | 0.00      | M                 | M13                |
| MCPS-064  | 05:06:45.79                | -67:18:23.9                | 16.706 ± 0.091 | 1.778 ± 0.104    | 271.83 ± 0.54                             | 0.00      | M                 | M13                |
| MCPS-066  | 05:06:50.42                | -67:17:35.3                | 16.561 ± 0.021 | 1.535 ± 0.032    | 273.43 ± 0.72                             | 0.00      | M                 | M13                |
| MCPS-067  | 05:06:51.17                | -67:36:00.7                | 16.463 ± 0.090 | 1.691 ± 0.104    | 294.50 ± 0.51                             | 0.00      | M                 | M13                |
| MCPS-070  | 05:06:53.80                | -67:38:02.3                | 16.586 ± 0.024 | 1.802 ± 0.047    | 226.58 ± 0.57                             | 0.00      | M                 | M13                |
| MCPS-071  | 05:06:57.88                | -67:17:13.5                | 16.403 ± 0.026 | 1.895 ± 0.036    | 260.83 ± 0.54                             | 0.00      | M                 | M13                |
| MCPS-074  | 05:07:01.90                | -67:19:20.7                | 16.718 ± 0.026 | 1.685 ± 0.036    | 287.22 ± 0.58                             | 0.00      | M                 | M13                |
| MCPS-075  | 05:07:03.10                | -67:19:53.2                | 16.650 ± 0.027 | 1.505 ± 0.037    | 237.56 ± 0.52                             | 0.00      | M                 | M13                |
| MCPS-076  | 05:07:07.28                | -67:35:51.3                | 16.745 ± 0.037 | 1.583 ± 0.054    | 263.83 ± 0.51                             | 0.00      | M                 | M13                |
| MCPS-078  | 05:07:10.43                | -67:37:17.1                | 16.799 ± 0.029 | 1.923 ± 0.050    | 310.96 ± 0.70                             | 0.00      | M                 | M13                |
| MCPS-079  | 05:07:10.53                | -67:39:57.4                | 16.680 ± 0.029 | 1.803 ± 0.049    | 290.05 ± 0.67                             | 0.00      | M                 | M13                |

Table 5 continued

Table 5 (continued)

| ID       | $\alpha_{2000}$<br>(h:m:s) | $\delta_{2000}$<br>(°:':") | $V$<br>(mag)   | $V - I$<br>(mag) | $v_{\text{los}}$<br>(km s <sup>-1</sup> ) | $P_{M_i}$ | Sel. <sup>a</sup> | Spec. <sup>b</sup> |
|----------|----------------------------|----------------------------|----------------|------------------|-------------------------------------------|-----------|-------------------|--------------------|
| MCPS-082 | 05:07:14.56                | -67:15:30.5                | 16.693 ± 0.031 | 1.532 ± 0.056    | 271.07 ± 0.62                             | 0.00      | M                 | M13                |
| MCPS-084 | 05:07:16.07                | -67:37:32.4                | 16.806 ± 0.025 | 1.832 ± 0.049    | 243.43 ± 0.65                             | 0.00      | M                 | M13                |
| MCPS-089 | 05:07:21.71                | -67:36:39.0                | 16.477 ± 0.116 | 1.639 ± 0.123    | 249.40 ± 0.45                             | 0.00      | M                 | M13                |
| MCPS-091 | 05:07:22.26                | -67:39:49.8                | 16.726 ± 0.026 | 1.877 ± 0.047    | 239.79 ± 0.55                             | 0.00      | M                 | M13                |
| MCPS-094 | 05:07:24.04                | -67:17:29.1                | 16.856 ± 0.026 | 1.610 ± 0.037    | 247.63 ± 0.54                             | 0.00      | M                 | M13                |
| MCPS-096 | 05:07:32.79                | -67:17:35.6                | 16.536 ± 0.046 | 1.857 ± 0.053    | 311.32 ± 0.55                             | 0.00      | M                 | M13                |
| MCPS-103 | 05:07:39.28                | -67:35:41.8                | 17.082 ± 0.027 | 1.747 ± 0.065    | 235.06 ± 0.51                             | 0.00      | M                 | M13                |
| MCPS-105 | 05:07:39.88                | -67:17:38.0                | 16.556 ± 0.022 | 1.759 ± 0.033    | 277.58 ± 0.59                             | 0.00      | M                 | M13                |
| MCPS-106 | 05:07:42.05                | -67:17:05.5                | 16.899 ± 0.027 | 1.682 ± 0.037    | 243.45 ± 0.55                             | 0.00      | M                 | M13                |
| MCPS-111 | 05:07:47.94                | -67:23:11.2                | 16.599 ± 0.031 | 2.012 ± 0.084    | 242.68 ± 0.76                             | 0.00      | M                 | M13                |
| MCPS-118 | 05:07:56.13                | -67:17:51.5                | 16.802 ± 0.029 | 1.600 ± 0.038    | 299.40 ± 0.49                             | 0.00      | M                 | M13                |
| MCPS-124 | 05:08:04.86                | -67:36:10.0                | 16.670 ± 0.063 | 1.517 ± 0.075    | 262.77 ± 0.43                             | 0.00      | M                 | M13                |
| MCPS-126 | 05:08:06.77                | -67:37:28.2                | 16.775 ± 0.023 | 1.923 ± 0.045    | 234.44 ± 0.60                             | 0.00      | M                 | M13                |
| MCPS-135 | 05:08:12.78                | -67:31:37.0                | 16.569 ± 0.024 | 1.596 ± 0.049    | 289.09 ± 0.43                             | 0.00      | M                 | M13                |
| MCPS-136 | 05:08:13.09                | -67:36:51.6                | 16.827 ± 0.025 | 1.533 ± 0.047    | 272.33 ± 0.45                             | 0.00      | M                 | M13                |
| MCPS-137 | 05:08:15.20                | -67:26:49.6                | 16.691 ± 0.031 | 1.788 ± 0.051    | 230.93 ± 0.46                             | 0.00      | M                 | M13                |
| MCPS-139 | 05:08:17.64                | -67:18:24.2                | 16.776 ± 0.070 | 1.819 ± 0.074    | 297.20 ± 0.57                             | 0.00      | M                 | M13                |
| MCPS-141 | 05:08:18.66                | -67:36:10.6                | 16.450 ± 0.023 | 1.823 ± 0.044    | 259.56 ± 0.56                             | 0.00      | M                 | M13                |
| MCPS-142 | 05:08:18.82                | -67:24:53.9                | 16.607 ± 0.028 | 1.596 ± 0.048    | 254.21 ± 0.42                             | 0.00      | M                 | M13                |
| MCPS-154 | 05:08:30.01                | -67:32:33.1                | 16.503 ± 0.040 | 1.968 ± 0.056    | 231.60 ± 0.74                             | 0.00      | M                 | M13                |
| MCPS-156 | 05:08:31.03                | -67:27:46.8                | 16.919 ± 0.036 | 1.573 ± 0.054    | 292.88 ± 0.48                             | 0.00      | M                 | M13                |
| MCPS-157 | 05:08:32.98                | -67:35:42.9                | 16.337 ± 0.040 | 1.803 ± 0.055    | 268.78 ± 0.64                             | 0.00      | M                 | M13                |
| MCPS-161 | 05:08:37.12                | -67:18:36.6                | 16.361 ± 0.024 | 1.900 ± 0.033    | 237.30 ± 0.58                             | 0.00      | M                 | M13                |
| MCPS-162 | 05:08:37.53                | -67:31:24.6                | 16.693 ± 0.028 | 1.805 ± 0.052    | 278.47 ± 0.54                             | 0.00      | M                 | M13                |
| MCPS-165 | 05:08:40.05                | -67:26:05.8                | 16.696 ± 0.023 | 1.632 ± 0.045    | 311.85 ± 0.42                             | 0.00      | M                 | M13                |
| MCPS-166 | 05:08:40.29                | -67:33:48.8                | 16.452 ± 0.028 | 1.924 ± 0.048    | 266.18 ± 0.69                             | 0.00      | M                 | M13                |
| MCPS-167 | 05:08:40.51                | -67:29:19.9                | 16.753 ± 0.027 | 1.623 ± 0.048    | 285.36 ± 0.55                             | 0.00      | M                 | M13                |
| MCPS-168 | 05:08:41.70                | -67:20:13.9                | 16.658 ± 0.023 | 2.008 ± 0.034    | 212.62 ± 0.70                             | 0.00      | M                 | M13                |
| MCPS-172 | 05:08:47.60                | -67:26:05.4                | 16.397 ± 0.032 | 1.563 ± 0.053    | 295.20 ± 0.50                             | 0.00      | M                 | M13                |
| MCPS-176 | 05:08:51.75                | -67:37:12.3                | 16.757 ± 0.179 | 1.695 ± 0.184    | 307.53 ± 0.65                             | 0.00      | M                 | M13                |
| MCPS-183 | 05:09:01.66                | -67:35:30.0                | 16.708 ± 0.028 | 1.999 ± 0.051    | 299.60 ± 0.71                             | 0.00      | M                 | M13                |
| MCPS-184 | 05:09:01.74                | -67:26:12.7                | 16.475 ± 0.026 | 1.828 ± 0.047    | 255.23 ± 0.54                             | 0.00      | M                 | M13                |
| MCPS-189 | 05:09:05.46                | -67:32:01.8                | 16.803 ± 0.045 | 1.554 ± 0.060    | 284.73 ± 0.65                             | 0.00      | M                 | M13                |
| MCPS-190 | 05:09:06.14                | -67:31:15.8                | 16.582 ± 0.027 | 1.617 ± 0.055    | 340.95 ± 0.46                             | 0.00      | M                 | M13                |
| MCPS-193 | 05:09:09.03                | -67:35:05.2                | 16.876 ± 0.034 | 1.589 ± 0.052    | 268.29 ± 0.72                             | 0.00      | M                 | M13                |
| MCPS-195 | 05:09:11.76                | -67:26:26.7                | 16.732 ± 0.090 | 1.577 ± 0.099    | 240.95 ± 0.54                             | 0.00      | M                 | M13                |
| MCPS-200 | 05:09:25.37                | -67:30:22.9                | 16.646 ± 0.036 | 1.485 ± 0.054    | 243.73 ± 0.60                             | 0.00      | M                 | M13                |

<sup>a</sup>Photometric source that the target were selected from: H stands for *HST* and M stands for MCPS.

<sup>b</sup>Spectroscopic source the LOS velocities were measured from: M2FS stands for this work, M13 stands for Mackey et al. (2013), and COMB stands for combined.
